# Supplementary material for: 4Real-Video: Learning Generalizable Photo-Realistic 4D Video Diffusion
Source: arXiv:2412.04462 source file (2024-12-05)
Supplement: Supplementary file 1 [file appendix.tex]

\noindent\textbf{Notaions}: 
\begin{itemize}
    \item $\mathbf{x}_t$, position of a point in the global coordinate at time $t$.
    \item $\mathbf{x}_c$, position of a point at canonical coordinate.
    \item $\mathbf{x}'_v$, position of a point from 3D tracking under $v$-th camera coordinate.
    \item $\mathbf{x}_{t,v}$, position of a point at time $t$ under $v$-th camera coordinate.
    \item $\mathbf{A}_{v}$, rigid transformation from canonical coordinate to $v$-th view.
    \item $s_v$, scale which aligns canonical coordiate to $v$-th view.
\end{itemize}

\noindent\textbf{Defination of deformation:}

\noindent\textbf{In canonical coordinate}
\begin{equation}
    \mathbf{x}_t = \mathbf{x}_c + \Delta \mathbf{x}_t
\end{equation}

\noindent\textbf{In view coordinate}
\begin{equation}
    \mathbf{x}_{t,v} = \mathbf{A}_{v} (\mathbf{x}_c + \Delta \mathbf{x}_t + \Delta \mathbf{x}_v)
    = \mathbf{A}_{v} (\mathbf{x}_c + \Delta \mathbf{x}_v) + \mathbf{A}_{v}\Delta \mathbf{x}_t
\end{equation}

\noindent\textbf{Review glabal alignment is Dust3R / Monst3R}
Since in global alignment, we are solving for $\mathbf{x}_c$, $\mathbf{A}_{v}$, $s_v$, such that minimizes the cost function (dropping unrelevant terms)
\begin{equation}
    \min \| \mathbf{x}_c - s_v^{-1} \mathbf{A}_{v}^{-1}  \mathbf{x}'_v \|
\end{equation},
therefore, we assume the residue view-dependent motion $\Delta \mathbf{x}_v$ satisfies:
\begin{equation}
    \mathbf{x}_c + \Delta \mathbf{x}_v = s_v^{-1} \mathbf{A}_{v}^{-1}  \mathbf{x}'_v
\end{equation}

\noindent\textbf{Finally}, this means in eq(2), we will have:
\begin{equation}
    \mathbf{x}_{t,v} = s_v^{-1}  \mathbf{x}'_v + \mathbf{A}_{v}\Delta \mathbf{x}_t
\end{equation}
On the right-hand-side, only $\Delta \mathbf{x}_t$ is unkown which you need to optimize given rendering losses.
